# Supplementary material for: Global-Lens Transformers: Adaptive Token Mixing for Dynamic Link Prediction
Source: arXiv:2511.12442 source file (2025-11-16)
Supplement: Supplementary file 1 [file Appendix.tex]

\appendix
\section{Appendix}
 \begin{table*}[]
\centering
\caption{Information about datasets.}
\label{tab:info datasets}
\resizebox{\textwidth}{!}
{
\setlength{}{}
{

\begin{tabular}{c|cccccccc}
\hline
Datasets  & Domains     & \#Nodes & \#Links   & \#N\&L Feat & Bipartite & Duration   & Unique Steps   & Time Granularity  \\ \hline
Wikipedia & Social      & 9,227   & 157,474   & –\& 172     & True      & 1  month   & 152,757      & Unix timestamps   \\
Reddit    & Social      & 10,984  & 672,447   & –\& 172     & True      & 1  month   & 669,065      & Unix timestamps   \\
MOOC      & Interaction & 7,144   & 411,749   & –\& 4       & True      & 17  months & 345,600      & Unix timestamps   \\
LastFM    & Interaction & 1,980   & 1,293,103 & –\& –       & True      & 1  month   & 1,283,614    & Unix timestamps   \\
SocialEvo       & Proximity      & 74   &  2,099,519    & –\& 2        & False     & 8 months  & 565,932       & Unix timestamps   \\ 
Enron     & Social      & 184     & 125,235   & –\& –       & False     & 3  years   & 22,632       & Unix timestamps    \\ \hline
\end{tabular}
}}
\end{table*}

\subsection{Datasets and Baselines.}
\textbf{Datasets.} The statistics for these datasets are summarized in \tabref{tab:info datasets}, where "\#N\&L Feat" denotes the dimensions of node and link features. Below is a comprehensive overview of each dataset.

\begin{itemize}
\item \textbf{Wikipedia}: 
Wikipedia captures interactions between users and pages on the platform. Each link is assigned a 172-dimensional feature from the Linguistic Inquiry and Word Count (LIWC).

\item \textbf{Reddit}: 
Reddit tracks the posts made by users in subreddits over one month. Each link is associated with a 172-dimensional feature from the Linguistic Inquiry and Word Count (LIWC).

\item \textbf{MOOC}: 
MOOC records the students' engagement with different course content units such as videos and problems. Each link is associated with a 4-dimensional feature. 

\item \textbf{LastFM}: 
The LastFM dataset captures user listening behavior over one month, recording connections between users and songs.

\item \textbf{Social Evo.}: The Social Evo dataset monitors the daily activities of an entire undergraduate dormitory for a period of eight months, where each link has a 2-dimensional feature.

\item \textbf{Enron}: 
The Enron dataset collects the email exchanges between employees in the Enron Corporation over a three-year period. 

\end{itemize}

\textbf{Backbones.} The descriptions of backbones are shown as follows.
\begin{itemize}
\item \textbf{TGN}: TGN \cite{DBLP:journals/corr/abs-2006-10637} handles dynamic graphs by maintaining evolving node memories, updated upon interactions via a message function, aggregator, and memory updater. A temporal attention module generates node representations for prediction.

\item \textbf{TCL}: TCL \cite{DBLP:journals/corr/abs-2105-07944} generates interaction sequences using breadth-first search on graphs, and employs a graph transformer with cross-attention to capture dependencies between nodes.

\item \textbf{TGAT}:  TGAT \cite{DBLP:conf/iclr/XuRKKA20} uses a self-attention mechanism to aggregate features from temporal neighbors and applies time encoding to capture temporal patterns from the sequences.

\item \textbf{CAWN}: CAWN \cite{DBLP:conf/iclr/WangCLL021} samples causal anonymous walks to model dynamics and node identities, encoding walks via recurrent neural networks and using self-attention to capture temporal patterns.

\item \textbf{DyGFormer}: DyGFormer \cite{DBLP:conf/nips/0004S0L23} encodes source-target relationships via neighbor co-occurrence and uses a patching strategy with Transformers to learn from long-term histories efficiently.
\end{itemize}

\subsection{Experiment Settings.}
\label{number of tokens}
The number of sampled neighbors and the number of neighbors for aggregations in each layer in GLFormer are shown in \tabref{tab:number of neighbors} and \tabref{tab:number of layer}, respectively.

% The number of sampled neighbors and the number of neighbors for aggregations in each layer in GLFormer are shown in \tabref{tab:number of layer}.

\begin{table}[!htbp]
\caption{Configurations of the number of sampled neighbors, the number of causal anonymous walks, and the length of input sequences \& the patch size of different methods.}
\label{tab:number of neighbors}
\resizebox{\columnwidth}{!}
{
\setlength{}{}
{
\begin{tabular}{c|ccccc}
\hline
Datasets  & TGAT & TGN & CAWN & TCL & DyGFormer \\ \hline
Wikipedia &  20 & 10 & 32 & 20 & 32\&1\\ 
Reddit & 20 & 10 & 32 & 20 & 64\&2 \\
MOOC & 20 & 10 & 64 & 20 & 256\&8\\
LastFM & 20 & 10 & 128 & 20 & 128\&16\\
SocialEvo & 20 & 10 & 64 & 20 & 32\&1 \\ 
Enron & 20 & 10 & 32 & 20 & 256\&8\\ \hline
\end{tabular}
}}
\end{table}

\begin{table}[!htbp]
\caption{Configurations for the number of layers in GLFormer and the corresponding number of neighbors used for aggregation in each layer.}
\label{tab:number of layer}
\resizebox{\columnwidth}{!}
{
\setlength{}{}
{
\begin{tabular}{c|cccccc}
\hline
\multirow{2}{*}{Methods} & \multicolumn{6}{c}{Datasets}                                                                                                                                                                           \\ \cline{2-7} 
                         & \multicolumn{1}{c|}{Wikipedia}     & \multicolumn{1}{c|}{Reddit}        & \multicolumn{1}{c|}{MOOC}          & \multicolumn{1}{c|}{LastFM}        & \multicolumn{1}{c|}{SocialEvo}     & Enron         \\ \hline
TGN                      & \multicolumn{1}{c|}{{[}2, 4, 8{]}} & \multicolumn{1}{c|}{{[}2, 4, 8{]}} & \multicolumn{1}{c|}{{[}2, 4, 8{]}} & \multicolumn{1}{c|}{{[}2, 4, 8{]}} & \multicolumn{1}{c|}{{[}2, 4, 8{]}} & {[}2, 4, 8{]} \\ \hline
TCL                      & \multicolumn{1}{c|}{{[}2, 4, 8{]}} & \multicolumn{1}{c|}{{[}2, 4, 8{]}} & \multicolumn{1}{c|}{{[}2, 4, 8{]}} & \multicolumn{1}{c|}{{[}2, 4, 8{]}} & \multicolumn{1}{c|}{{[}2, 4, 8{]}} & {[}2, 4, 8{]} \\ \hline
TGAT                     & \multicolumn{1}{c|}{{[}2, 4{]}}    & \multicolumn{1}{c|}{{[}2, 4{]}}    & \multicolumn{1}{c|}{{[}2, 4{]}}    & \multicolumn{1}{c|}{{[}2, 4{]}}    & \multicolumn{1}{c|}{{[}2, 4{]}}    & {[}2, 4{]}    \\ \hline
CAWN                     & \multicolumn{1}{c|}{{[}2, 4{]}}    & \multicolumn{1}{c|}{{[}2, 4{]}}    & \multicolumn{1}{c|}{{[}2, 4{]}}    & \multicolumn{1}{c|}{{[}2, 4{]}}    & \multicolumn{1}{c|}{{[}2, 4{]}}    & {[}2, 4{]}    \\ \hline
DyGFormer                & \multicolumn{1}{c|}{{[}2, 4, 8{]}} & \multicolumn{1}{c|}{{[}2, 4, 8{]}} & \multicolumn{1}{c|}{{[}2, 4, 8{]}} & \multicolumn{1}{c|}{{[}2, 4, 8{]}} & \multicolumn{1}{c|}{{[}2, 4, 8{]}} & {[}2, 4, 8{]} \\ \hline
\end{tabular}
}}
\end{table}

\subsection{Effectiveness of the Framework.}
The AUC-ROC results in different numbers of GLFormer are shown in \figref{fig:trans auc}.

 \begin{figure}[h!]
    \centering
\includegraphics[width=1.0\columnwidth]{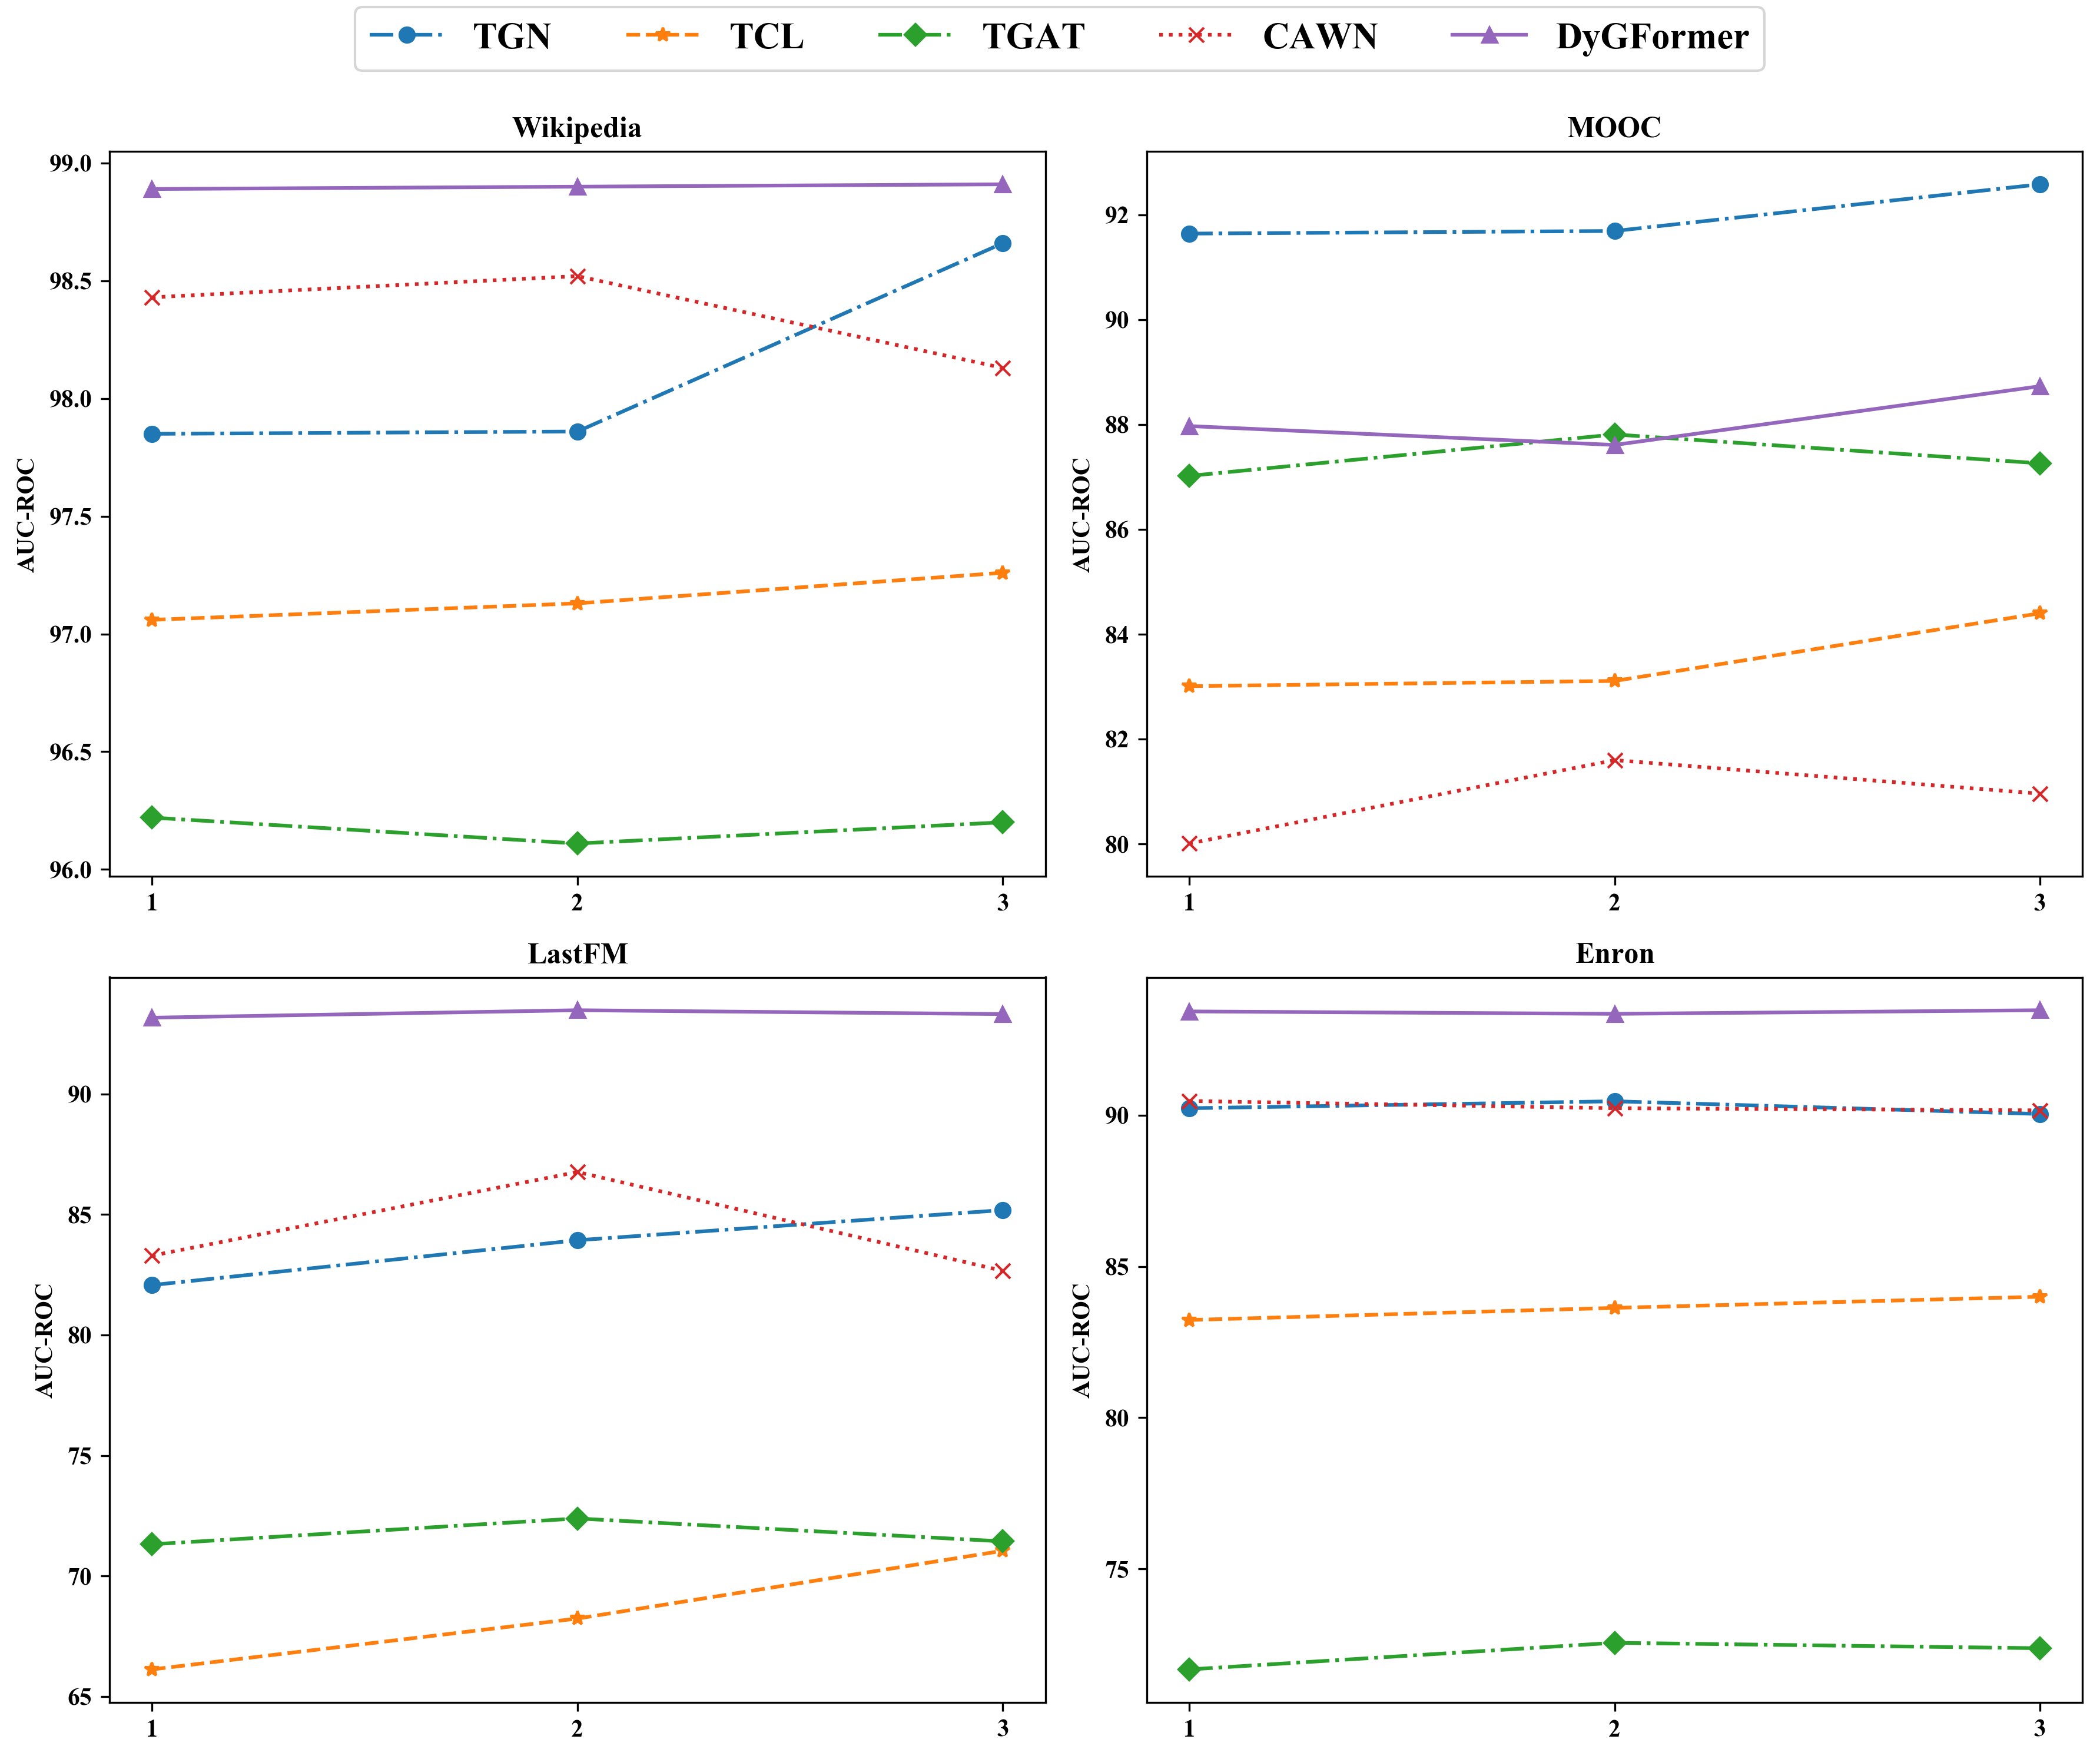}
    \caption{AUC-ROC in different GLFormer layers in transductive dynamic link prediction.}
    \label{fig:trans auc}
\end{figure}

\subsection{Ablation Study.}
The AUC-ROC results for different components in our framework are shown in \figref{fig:ablation trans auc}.

 \begin{figure}[h!]
    \centering
\includegraphics[width=1.0\columnwidth]{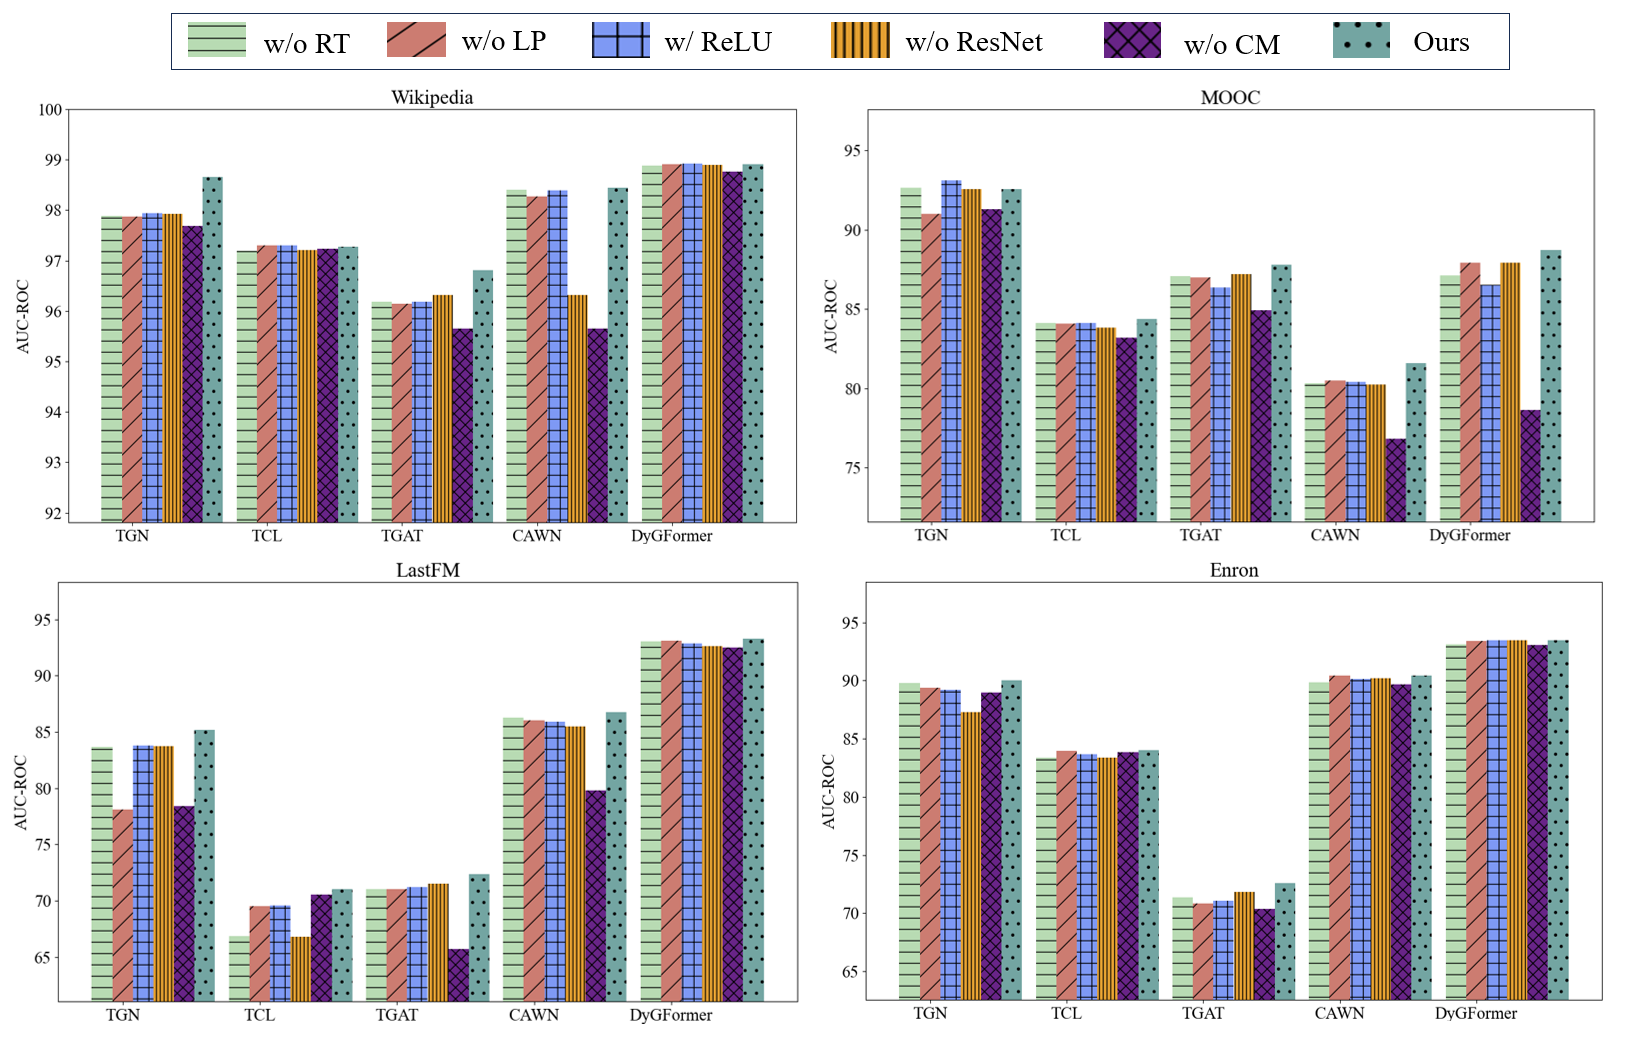}
    \caption{AUC-ROC for different components in transductive dynamic link prediction.}
    \label{fig:ablation trans auc}
\end{figure}

\subsection{Performance in inductive dynamic link prediction.}
\label{ref:total performance}
We show the performance of AP and AUC in inductive link prediction in \tabref{inductive}.

\begin{table*}[ht]
\caption{Performance for inductive dynamic link prediction on datasets.}
\label{inductive}
\resizebox{\textwidth}{!}
{
\setlength{}{}
{
\begin{tabular}{c|c|c|cccccc|c}
\hline
\multirow{2}{*}{Metric}   & \multirow{2}{*}{Backbone}  & \multirow{2}{*}{Method} & \multicolumn{6}{c|}{Datasets}                                                                                                                                                                                                                                    & \multirow{2}{*}{Rank} \\ \cline{4-9}
                          &                            &                         & \multicolumn{1}{c|}{Wikipedia}             & \multicolumn{1}{c|}{Reddit}                  & \multicolumn{1}{c|}{MOOC}                    & \multicolumn{1}{c|}{LastFM}                  & \multicolumn{1}{c|}{SocialEvo}               & Enron                   &                       \\ \hline
\multirow{20}{*}{AP}      & \multirow{4}{*}{TGN}       & Vanilla                   & \multicolumn{1}{c|}{97.77 ±   0.08}        & \multicolumn{1}{c|}{97.50 ±   0.07}          & \multicolumn{1}{c|}{89.04 ±   1.17}          & \multicolumn{1}{c|}{81.45 ±   4.29}          & \multicolumn{1}{c|}{90.77 ± 0.86}            & 78.52 ±   2.21          & 3.17                  \\
                          &                            & Pooling                    & \multicolumn{1}{c|}{97.53 ± 0.22}          & \multicolumn{1}{c|}{\textbf{97.58 ± 0.04}}   & \multicolumn{1}{c|}{91.41 ± 0.57}            & \multicolumn{1}{c|}{88.45 ± 1.07}            & \multicolumn{1}{c|}{\textbf{91.50 ± 0.19}}   & 78.52 ± 2.57            & \textbf{2.17}         \\
                          &                            & MLP                     & \multicolumn{1}{c|}{\textbf{97.82 ± 0.09}} & \multicolumn{1}{c|}{97.23 ± 0.15}            & \multicolumn{1}{c|}{\textbf{91.45 ± 0.60}}   & \multicolumn{1}{c|}{\textbf{89.51 ± 0.96}}   & \multicolumn{1}{c|}{90.76 ± 0.51}            & 78.84 ± 2.12            & \textbf{2.17}         \\
                          &                            & GLFormer              & \multicolumn{1}{c|}{97.51 ± 0.10}          & \multicolumn{1}{c|}{97.51 ±   0.10}          & \multicolumn{1}{c|}{89.90 ±   0.56}          & \multicolumn{1}{c|}{88.50 ±   1.39}          & \multicolumn{1}{c|}{91.40 ± 0.49}            & \textbf{80.76 ± 1.56}   & 2.33                  \\ \cline{2-10} 
                          & \multirow{4}{*}{TCL}       & Vanilla                   & \multicolumn{1}{c|}{96.22 ± 0.17}          & \multicolumn{1}{c|}{94.09 ± 0.07}            & \multicolumn{1}{c|}{80.60 ±   0.22}          & \multicolumn{1}{c|}{\textbf{73.53 ± 1.66}}   & \multicolumn{1}{c|}{91.55 ± 0.09}            & 76.14 ±   0.79          & 3.67                  \\
                          &                            & Pooling                    & \multicolumn{1}{c|}{94.77 ± 0.07}          & \multicolumn{1}{c|}{94.35 ± 0.12}            & \multicolumn{1}{c|}{79.38 ±   0.51}          & \multicolumn{1}{c|}{75.96 ± 5.48}            & \multicolumn{1}{c|}{92.26 ± 0.07}            & 82.94 ±   0.68          & 3.17                  \\
                          &                            & MLP                     & \multicolumn{1}{c|}{97.45 ± 0.07}          & \multicolumn{1}{c|}{\textbf{97.39 ± 0.19}}   & \multicolumn{1}{c|}{82.67 ±   1.22}          & \multicolumn{1}{c|}{79.28 ±   4.24}          & \multicolumn{1}{c|}{\textbf{92.55 ± 0.04}}   & 82.74 ±   0.45          & 1.83                  \\
                          &                            & GLFormer              & \multicolumn{1}{c|}{\textbf{97.51 ± 0.05}} & \multicolumn{1}{c|}{95.16 ± 0.08}            & \multicolumn{1}{c|}{\textbf{82.82 ±   1.60}} & \multicolumn{1}{c|}{\textbf{81.35 ±   2.03}} & \multicolumn{1}{c|}{{92.42 ± 0.18}}   & \textbf{83.05 ±   0.71} & \textbf{1.33}         \\ \cline{2-10} 
                          & \multirow{4}{*}{TGAT}      & Vanilla                   & \multicolumn{1}{c|}{96.22 ± 0.07}          & \multicolumn{1}{c|}{\textbf{97.09 ± 0.04}}   & \multicolumn{1}{c|}{85.50 ± 0.19}            & \multicolumn{1}{c|}{78.63 ± 0.31}            & \multicolumn{1}{c|}{91.41 ± 0.16}            & 67.05 ± 1.51            & 3.17                  \\
                          &                            & Pooling                    & \multicolumn{1}{c|}{96.21 ± 0.08}          & \multicolumn{1}{c|}{96.89 ± 0.04}            & \multicolumn{1}{c|}{85.91 ±   0.23}          & \multicolumn{1}{c|}{78.81 ± 0.14}            & \multicolumn{1}{c|}{91.80 ± 0.08}            & 65.46 ±   0.54          & 3.17                  \\
                          &                            & MLP                     & \multicolumn{1}{c|}{96.27 ± 0.15}          & \multicolumn{1}{c|}{96.83 ± 0.06}            & \multicolumn{1}{c|}{86.03 ±   0.40}          & \multicolumn{1}{c|}{\textbf{79.72 ± 0.27}}   & \multicolumn{1}{c|}{92.15 ± 0.24}            & 68.67 ±   0.24          & 2                     \\
                          &                            & GLFormer              & \multicolumn{1}{c|}{\textbf{96.35 ± 0.13}} & \multicolumn{1}{c|}{96.57 ± 0.09}            & \multicolumn{1}{c|}{\textbf{86.50 ±   0.08}} & \multicolumn{1}{c|}{79.66 ± 0.41}            & \multicolumn{1}{c|}{\textbf{93.23 ± 0.02}}   & \textbf{70.06 ±   0.92} & \textbf{1.67}         \\ \cline{2-10} 
                          & \multirow{4}{*}{CAWN}      & Vanilla                   & \multicolumn{1}{c|}{98.24 ± 0.03}          & \multicolumn{1}{c|}{98.62 ± 0.01}            & \multicolumn{1}{c|}{81.42 ±   0.24}          & \multicolumn{1}{c|}{89.42 ± 0.07}            & \multicolumn{1}{c|}{79.94 ± 0.18}            & 86.35 ± 0.51            & 3                     \\
                          &                            & Pooling                    & \multicolumn{1}{c|}{98.19 ± 0.06}          & \multicolumn{1}{c|}{98.56 ± 0.01}            & \multicolumn{1}{c|}{\textbf{83.49 ±   0.23}} & \multicolumn{1}{c|}{89.92  ±  0.11}          & \multicolumn{1}{c|}{79.78 ±   0.33}          & 86.99 ± 0.16            & 3                     \\
                          &                            & MLP                     & \multicolumn{1}{c|}{\textbf{98.37 ± 0.01}} & \multicolumn{1}{c|}{\textbf{98.64 ± 0.01}}   & \multicolumn{1}{c|}{83.47 ±   0.08}          & \multicolumn{1}{c|}{89.97  ±  0.03}          & \multicolumn{1}{c|}{\textbf{80.28 ± 0.29}}   & \textbf{87.17 ± 0.02}   & \textbf{1.33}         \\
                          &                            & GLFormer              & \multicolumn{1}{c|}{98.24 ± 0.11}          & \multicolumn{1}{c|}{98.58 ± 0.02}            & \multicolumn{1}{c|}{82.05 ±   0.13}          & \multicolumn{1}{c|}{\textbf{90.11 ± 0.24}}   & \multicolumn{1}{c|}{80.15 ± 0.12}            & 86.35 ± 0.51            & 2.33                  \\ \cline{2-10} 
                          & \multirow{4}{*}{DyGFormer} & Vanilla                   & \multicolumn{1}{c|}{{98.59 ± 0.03}} & \multicolumn{1}{c|}{98.84 ± 0.02}            & \multicolumn{1}{c|}{86.96 ± 0.43}            & \multicolumn{1}{c|}{94.23 ±   0.09}          & \multicolumn{1}{c|}{93.14 ± 0.04}            & 89.76 ±   0.34          & 2.83                  \\
                          &                            & Pooling                    & \multicolumn{1}{c|}{98.58 ± 0.04}          & \multicolumn{1}{c|}{98.45 ± 0.05}            & \multicolumn{1}{c|}{84.47 ±   0.38}          & \multicolumn{1}{c|}{94.35 ±   0.04}          & \multicolumn{1}{c|}{93.18 ± 0.02}            & 89.41 ±   0.09          & 3.5                   \\
                          &                            & MLP                     & \multicolumn{1}{c|}{98.59 ± 0.05}          & \multicolumn{1}{c|}{98.60 ± 0.07}            & \multicolumn{1}{c|}{84.82 ±   0.34}          & \multicolumn{1}{c|}{94.48 ±   0.03}          & \multicolumn{1}{c|}{93.18 ± 0.06}            & \textbf{89.85 ± 0.20}   & 2.17                  \\
                          &                            & GLFormer              & \multicolumn{1}{c|}{\textbf{98.64 ± 0.02}} & \multicolumn{1}{c|}{\textbf{98.86 ±   0.01}} & \multicolumn{1}{c|}{\textbf{87.26 ±   0.49}} & \multicolumn{1}{c|}{\textbf{94.51 ±   0.14}} & \multicolumn{1}{c|}{\textbf{93.23 ± 0.02}}   & 89.80 ± 0.06            & \textbf{1.17}         \\ \hline
\multirow{20}{*}{AUC-ROC} & \multirow{4}{*}{TGN}       & Vanilla                   & \multicolumn{1}{c|}{97.69 ±   0.08}        & \multicolumn{1}{c|}{97.39 ± 0.07}            & \multicolumn{1}{c|}{91.24 ±   0.99}          & \multicolumn{1}{c|}{82.61 ±   3.15}          & \multicolumn{1}{c|}{93.43 ± 0.59}            & 79.58 ±   2.74          & 3.17                  \\
                          &                            & Pooling                    & \multicolumn{1}{c|}{97.40 ± 0.23}          & \multicolumn{1}{c|}{\textbf{97.54 ± 0.04}}   & \multicolumn{1}{c|}{\textbf{93.04 ± 0.59}}   & \multicolumn{1}{c|}{88.54 ± 0.83}            & \multicolumn{1}{c|}{93.54 ± 0.08}            & 80.07 ± 2.12            & 2.17                  \\
                          &                            & MLP                     & \multicolumn{1}{c|}{\textbf{97.72 ± 0.10}} & \multicolumn{1}{c|}{97.24 ± 0.19}            & \multicolumn{1}{c|}{92.85 ± 0.57}            & \multicolumn{1}{c|}{\textbf{89.32 ± 1.01}}   & \multicolumn{1}{c|}{93.39 ± 0.22}            & 79.78 ± 2.42            & 2.5                   \\
                          &                            & GLFormer              & \multicolumn{1}{c|}{97.43 ± 0.13}          & \multicolumn{1}{c|}{97.43 ±   0.13}          & \multicolumn{1}{c|}{91.24 ±   0.53}          & \multicolumn{1}{c|}{88.56 ±   1.26}          & \multicolumn{1}{c|}{\textbf{93.63 ±   0.47}} & \textbf{82.14 ±   1.69} & \textbf{2}            \\ \cline{2-10} 
                          & \multirow{4}{*}{TCL}       & Vanilla                   & \multicolumn{1}{c|}{95.57 ± 0.20}          & \multicolumn{1}{c|}{93.80 ± 0.07}            & \multicolumn{1}{c|}{81.43 ±   0.19}          & \multicolumn{1}{c|}{70.84 ± 0.85}            & \multicolumn{1}{c|}{93.71 ± 0.18}            & 72.33 ±   0.99          & 3.67                  \\
                          &                            & Pooling                    & \multicolumn{1}{c|}{94.35 ± 0.11}          & \multicolumn{1}{c|}{94.14 ± 0.11}            & \multicolumn{1}{c|}{80.84 ±   0.44}          & \multicolumn{1}{c|}{72.34 ± 5.40}            & \multicolumn{1}{c|}{94.44± 0.12}             & 81.03 ±   1.07          & 3.17                  \\
                          &                            & MLP                     & \multicolumn{1}{c|}{96.99 ± 0.09}          & \multicolumn{1}{c|}{\textbf{97.37 ± 0.19}}   & \multicolumn{1}{c|}{82.79 ±   0.77}          & \multicolumn{1}{c|}{75.23 ±   3.15}          & \multicolumn{1}{c|}{\textbf{94.64 ± 0.01}}   & 80.93 ±   0.57          & 1.83                  \\
                          &                            & GLFormer              & \multicolumn{1}{c|}{\textbf{97.08 ± 0.09}} & \multicolumn{1}{c|}{94.74 ± 0.12}            & \multicolumn{1}{c|}{\textbf{83.00 ±   1.15}} & \multicolumn{1}{c|}{\textbf{76.88 ± 2.17}}   & \multicolumn{1}{c|}{94.54 ± 0.12}            & \textbf{81.63 ± 0.84}   & \textbf{1.33}         \\ \cline{2-10} 
                          & \multirow{4}{*}{TGAT}      & Vanilla                   & \multicolumn{1}{c|}{95.90 ± 0.09}          & \multicolumn{1}{c|}{\textbf{96.98 ± 0.04}}   & \multicolumn{1}{c|}{86.84 ± 0.17}            & \multicolumn{1}{c|}{76.99 ± 0.29}            & \multicolumn{1}{c|}{93.41 ± 0.19}            & 64.63 ± 1.74            & 3.33                  \\
                          &                            & Pooling                    & \multicolumn{1}{c|}{95.94 ± 0.11}          & \multicolumn{1}{c|}{96.78 ± 0.02}            & \multicolumn{1}{c|}{87.44 ±   0.27}          & \multicolumn{1}{c|}{77.14 ± 0.07}            & \multicolumn{1}{c|}{93.74 ± 0.12}            & 64.06 ±   0.61          & 3                     \\
                          &                            & MLP                     & \multicolumn{1}{c|}{96.04 ± 0.19}          & \multicolumn{1}{c|}{96.77 ± 0.04}            & \multicolumn{1}{c|}{87.53 ±   0.43}          & \multicolumn{1}{c|}{77.83  ± 0.14}           & \multicolumn{1}{c|}{94.32 ± 0.16}            & 65.12 ±   0.24          & 2.17                  \\
                          &                            & GLFormer              & \multicolumn{1}{c|}{\textbf{96.07 ± 0.13}} & \multicolumn{1}{c|}{96.43 ± 0.11}            & \multicolumn{1}{c|}{\textbf{87.71 ±   0.19}} & \multicolumn{1}{c|}{\textbf{78.05 ± 0.19}}   & \multicolumn{1}{c|}{\textbf{95.40 ± 0.03}}   & \textbf{66.92 ±   0.77} & \textbf{1.5}          \\ \cline{2-10} 
                          & \multirow{4}{*}{CAWN}      & Vanilla                   & \multicolumn{1}{c|}{98.03 ± 0.04}          & \multicolumn{1}{c|}{{98.42 ± 0.02}}   & \multicolumn{1}{c|}{81.86 ±   0.25}          & \multicolumn{1}{c|}{87.82 ± 0.12}            & \multicolumn{1}{c|}{84.73 ± 0.27}            & 87.02 ±   0.50          & 3                     \\
                          &                            & Pooling                    & \multicolumn{1}{c|}{97.94 ± 0.04}          & \multicolumn{1}{c|}{98.34 ± 0.01}            & \multicolumn{1}{c|}{\textbf{84.23 ±   0.25}} & \multicolumn{1}{c|}{87.92  ± 0.07}           & \multicolumn{1}{c|}{84.39 ±   0.19}          & 87.41 ± 0.28            & 3                     \\
                          &                            & MLP                     & \multicolumn{1}{c|}{\textbf{98.19 ± 0.04}} & \multicolumn{1}{c|}{\textbf{98.47 ± 0.03}}   & \multicolumn{1}{c|}{84.04 ±   0.17}          & \multicolumn{1}{c|}{88.47  ± 0.26}           & \multicolumn{1}{c|}{\textbf{85.22  ± 0.14}}  & \textbf{87.73 ± 0.13}   & \textbf{1.33}         \\
                          &                            & GLFormer              & \multicolumn{1}{c|}{97.97 ± 0.15}          & \multicolumn{1}{c|}{98.37 ± 0.02}            & \multicolumn{1}{c|}{82.68 ±   0.10}          & \multicolumn{1}{c|}{\textbf{88.70 ± 0.20}}   & \multicolumn{1}{c|}{85.06 ± 0.03}            & 87.02 ± 0.50            & 2.5                   \\ \cline{2-10} 
                          & \multirow{4}{*}{DyGFormer} & Vanilla                   & \multicolumn{1}{c|}{98.48 ± 0.03}          & \multicolumn{1}{c|}{98.71 ± 0.01}            & \multicolumn{1}{c|}{87.62 ± 0.51}            & \multicolumn{1}{c|}{94.08 ±   0.08}          & \multicolumn{1}{c|}{95.29 ± 0.03}            & 90.69 ±   0.26          & 2.83                  \\
                          &                            & Pooling                    & \multicolumn{1}{c|}{98.47 ± 0.03}          & \multicolumn{1}{c|}{98.27 ± 0.04}            & \multicolumn{1}{c|}{86.16 ±   0.29}          & \multicolumn{1}{c|}{94.21 ± 0.02}            & \multicolumn{1}{c|}{95.30 ± 0.06}            & 90.55 ± 0.16            & 3.5                   \\
                          &                            & MLP                     & \multicolumn{1}{c|}{98.48 ± 0.03}          & \multicolumn{1}{c|}{98.48 ± 0.09}            & \multicolumn{1}{c|}{86.07 ±   0.28}          & \multicolumn{1}{c|}{94.27 ±   0.05}          & \multicolumn{1}{c|}{95.33 ± 0.04}            & 90.76 ± 0.38            & 2.5                   \\
                          &                            & GLFormer              & \multicolumn{1}{c|}{\textbf{98.51 ± 0.02}} & \multicolumn{1}{c|}{\textbf{98.76 ±   0.01}} & \multicolumn{1}{c|}{\textbf{88.30 ±   0.59}} & \multicolumn{1}{c|}{\textbf{94.31 ± 0.12}}   & \multicolumn{1}{c|}{\textbf{95.40 ± 0.03}}   & \textbf{90.92 ± 0.10}   & \textbf{1}            \\ \hline
\end{tabular}
}}\end{table*}
